# Supplementary material for: Synthetic Landau levels for photons
Source: arXiv:1511.07381 source file (2017-01-24)
Supplement: Supplementary file 1 [file Schine-suppinfo_Revised_3.pdf]

# Supplementary Information


1. Details of the experimental apparatus
2. A brief introduction to magnetic fields, rotating systems, and Landau levels
3. Astigmatism drives only $\Delta L = 2$ transitions
4. Computing the mode spectrum of a general non-planar resonator
5. Understanding twisted resonators in the ray picture
6. Extracting Hamiltonian parameters for the twisted resonator
7. More on the Landau level structure of our resonator
8. Invariance under magnetic translations of the lowest Landau level modes in the Laguerre-Gauss basis
9. The form of the N-particle bosonic Laughlin state on a cone
    a. Away from the cone tip
    b. At the cone tip
    c. Experimental considerations
10. Comparison to the proposal of Umucalılar and Carusotto
11. Measurable quantities of quantum Hall systems: topological shift and trapped fractional charge
12. The local density of states and flux threaded cones
13. Twisting light: other methods to cause a 2D rotation of light
    a. Astigmatic three-mirror resonator
    b. Twisting waveguide
    c. Writhing waveguide
14. A note on time reversal symmetry in our system


**1. Details of the experimental apparatus** Two 780 nm optical paths are combined and mode matched into the experimental resonator. The first is the output of a digital micromirror device (DMD) for arbitrary mode injection. The second is the output of a fiber-coupled electro-optic modulator (EOM). This is coupled only to the $l = 0$ resonator mode. By looking at the transmission signal on an avalanche photodiode and tuning the EOM modulation frequency until the $l = 0$ sideband overlaps with the desired mode, we may read off the mode spacing as precisely that modulation frequency. This avoids the need to calibrate the non-linear scan of the piezo. As the mode indices become large, aberrations in the DMD and subsequent optics limit coupling of power into the desired mode. Additionally, a CCD camera in transmission captures images of the resonator's transverse mode profiles.

For mode injection into our resonator, we employ a DLP LightCrafter Module using the DLP3000 DMD with 608 by 684 square aluminum mirrors, 7.6 μm in side length, with a filling factor of 92% and reflectivity R ~ 90% at our operating wavelength of 780 nm. To achieve control over both amplitude and phase, the DMD mirrors create a hologram producing a diffraction pattern. We then send the first order fringe into the resonator. Following the techniques set forth by Zupancic[31], we image the diffraction off a DMD hologram into a Fourier plane of the DMD and calculate a phase map correction to reduce aberrations in the DMD image. We find such maps correct smoothly varying phase errors with a deviation magnitude of $2.8 \times 2\pi$ across the DMD chip.

The mirrors used in the experimental resonator have a high-reflectivity dielectric coating providing 0.0028% transmission at 780 nm. Our narrow 780 nm source has a linewidth $\kappa \approx 10$ kHz, and is locked to a reference cavity produced by Stable Laser Systems. The resonator mirrors are mounted in a 3D printed plastic structure. Coarse resonator length adjustment is provided by a micrometer translation stage, while fine adjustment is provided by piezo actuators mounted behind two of the mirrors. The experimental setup, along with photographs of the experimental resonator, is represented in Fig. S1.

**2. A brief introduction to magnetic fields, rotating systems, and Landau levels** Electrons confined in two dimensions and subjected to a constant perpendicular magnetic $\boldsymbol{B}=B\boldsymbol{z}$ experience the minimal coupling Hamiltonian, which may be written in terms of the particle momentum $\boldsymbol{p}$, electron charge e and mass m, as well as the angular momentum $\boldsymbol{L}$ and a vector potential $\boldsymbol{A}$(r) defined according to $\boldsymbol{\nabla} \times \boldsymbol{A} = \boldsymbol{B}$:

$$H = \frac{(\boldsymbol{p} - e\boldsymbol{A})^2}{2m} = \frac{\boldsymbol{p}^2}{2m} - \frac{eB}{2m}\boldsymbol{L_z} + \frac{(eB)^2}{8m}r^2$$

where the second equality follows from utilizing the symmetric gauge for the vector potential of a uniform magnetic field. In continuum systems, such a magnetic field gives rise to flat bands (Landau levels) and the quantum Hall effect[32], while in periodically modulated systems the generically chaotic Hofstadter butterfly spectrum results[33,34]. In both cases the system exhibits topologically protected mid-gap edge-channels characteristic of the broader family of topological insulators[35].

While an *actual* magnetic field only acts in this way on a charged particle, synthetic magnetic fields have been realized in charge-neutral systems; employing Raman couplings for cold atomic

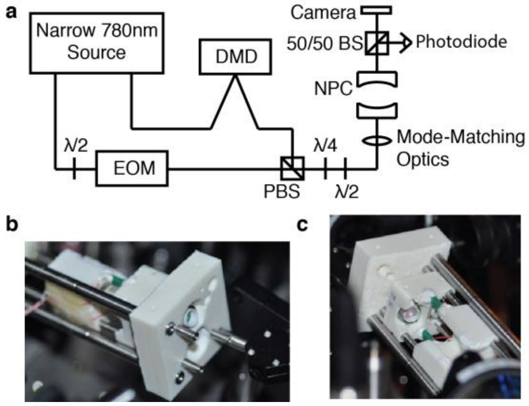


**Figure S1. a,** A schematic of the experimental setup is shown. Two beams from a 780 nm laser with a ~10 kHz linewidth are used. One reflects off a digital micromirror device while a second passes through an electro-optic modulator before being combined on a polarizing beam splitter. Two waveplates and mode matching optics allow coupling into a single circularly-polarized mode of the resonator; the reference beam couples into the (0,0) modes while the DMD beam couples into any mode as determined by the hologram projected onto the DMD surface. The transmitted light is collected on a camera and a photodiode. **b-c,** Photographs of the front (**b**) and back (**c**) of the experimental resonator show mirrors in stainless steel holders imbedded in two 3D printed plastic mounts. Two piezos (green) move the smaller, back mount along rails to vary the resonator round trip length. (Photographs by N.S.)

gases[36] and by "spinning up"[29,37,38] superfluids of helium and cold atoms. The latter approach makes use of the fact that in a frame rotating with angular velocity $\boldsymbol{\Omega}$, there arises an $\boldsymbol{\Omega} \cdot \boldsymbol{L}$ **term** in the Hamiltonian[39]:

$$H = \frac{\boldsymbol{p}^2}{2m} - \boldsymbol{\Omega} \cdot \boldsymbol{L}$$

$$= \frac{(\boldsymbol{p} - e\boldsymbol{A})^2}{2m} - \frac{|eA|^2}{2m}$$

Thus the rotating frame Hamiltonian is equivalent to a magnetic field $\boldsymbol{B} = \boldsymbol{\nabla} \times \boldsymbol{A} = \frac{e\boldsymbol{\Omega}}{2m}$ plus a centrifugal anti-confining potential in the plane orthogonal to $\boldsymbol{\Omega}$ : $V_{rot} = -\frac{1}{2} m\Omega^2 r_\perp^2$ [10]. It has thus been possible to stir a superfluid and observe the appearance of quantized vortices[29,38] that crystallize into Abrikosov lattices. Such lattices are predicted to melt into fractional quantum hall states as the particle density drops in a 2D system[40], but it has thus far been impossible to realize sufficiently strong interactions at sufficiently low densities.

**3. Astigmatism drives only $\Delta L = 2$ transitions** Astigmatism causes particle loss in a degenerate set by boundlessly increasing particles' angular momentum. We show here that the increase in angular momentum comes in steps of two. This underpins the stability of modes of in our resonator in which degenerate sets include only every third angular momentum state.

From definitions of ladder operators, $\hat{x} = \sqrt{\frac{\hbar}{2m\omega}}\left(\hat{a}_x + \hat{a}_x^\dagger\right)$, $\hat{a}_R = \frac{1}{2}\left(\hat{a}_x + i\hat{a}_y\right)$, $\hat{a}_L = \frac{1}{2}(\hat{a}_x - i\hat{a}_y)$ where $\hat{a}_R^\dagger$ increases angular momentum by one while $\hat{a}_L^\dagger$ decreases angular momentum by one,

$$\hat{x} = \sqrt{\frac{\hbar}{8m\omega}}\left(\hat{a}_R + \hat{a}_L + \hat{a}_R^\dagger + \hat{a}_L^\dagger\right) \text{ and } \hat{y} = -i\sqrt{\frac{\hbar}{8m\omega}}\left(\hat{a}_R - \hat{a}_L - \hat{a}_R^\dagger + \hat{a}_L^\dagger\right).$$

Astigmatism introduces a potential of the form $x^2 - y^2$, and so we rewrite this in terms of our angular momentum ladder operators to find

$$\hat{x}^2 - \hat{y}^2 = \frac{\hbar}{4m\omega}\left(\hat{a}_R^2 + \hat{a}_L^2 + (\hat{a}_R^\dagger)^2 + \left(\hat{a}_L^\dagger\right)^2 + 2\hat{a}_R\hat{a}_L^\dagger + 2\hat{a}_R^\dagger\hat{a}_L\right)$$

This clearly drives only $\Delta L = 2$ transitions.

**4. Computing the mode spectrum of a general non-planar resonator** The mode spectrum of an arbitrary $n$-mirror non-planar resonator may be computed by employing a 4x4 generalization[41] of the ABCD matrix formalism. We assume spherical mirrors but do account for astigmatism from non-normal incidence. The essential addition beyond the calculation for planar systems is the necessity to carry along a coordinate-system with us as we traverse the resonator. While coordinate transformations can be gauged away within a round-trip, we must start the next round-trip in the same coordinate system that we concluded the prior, so the rotation induced by non-planar reflections cannot be gauged away. This is analogous to a Berry/Aharanov-Bohm phase acquired upon hopping around a plaquette in an optical lattice[42,43].

In our resonator the mirrors are all spherical but are rendered effectively astigmatic by non-normal reflections[41]. Because the astigmatism is (by definition) diagonal in the sagittal-tangential basis, it is convenient to employ this as a coordinate system at each mirror reflection, and perform coordinate rotations to remain in this basis for each mirror as we traverse the resonator.

For a resonator whose $n$ mirrors are at locations $\boldsymbol{x}_j$, with radius of curvature $ROC_j$, we define the following quantities (assuming that the beam propagates through the resonator in increasing order of mirror index, and for simplicity that the indices repeat at $j=n$). We further assume that the mirrors have themselves been oriented so that the axis of the resonator passes through the $\boldsymbol{x}_j$.

The vectors connecting sequential mirrors are

$$\boldsymbol{M}_{ij} = \boldsymbol{x}_i - \boldsymbol{x}_j, \quad \boldsymbol{m}_{ij} = \frac{\boldsymbol{M}_{ij}}{|\boldsymbol{M}_{ij}|}.$$

A vector normal to the plane of propagation in the plane of the mirror surface is

$$\boldsymbol{n}_j = \frac{\boldsymbol{m}_{j,j-1} \times \boldsymbol{m}_{j,j+1}}{|\boldsymbol{m}_{j,j-1} \times \boldsymbol{m}_{j,j+1}|}.$$

From these we define a propagation coordinate system before *(IN)* and after *(OUT)* the reflection off of mirror $j$, normal to the direction of propagation.

$$\boldsymbol{x}_j^{IN} = \boldsymbol{n}_j, \quad \boldsymbol{x}_j^{OUT} = \boldsymbol{n}_j$$

$$\boldsymbol{y}_j^{IN} = \frac{\boldsymbol{n}_j \times \boldsymbol{m}_{j,j-1}}{|\boldsymbol{n}_j \times \boldsymbol{m}_{j,j-1}|}, \quad \boldsymbol{y}_j^{OUT} = \frac{\boldsymbol{n}_j \times \boldsymbol{m}_{j,j+1}}{|\boldsymbol{n}_j \times \boldsymbol{m}_{j,j+1}|}$$

We are now prepared to compute the rotation matrix that transforms from the coordinate system after mirror $j$ to that before mirror $j$+1.

$$\mathbf{R}_j = \begin{pmatrix} \boldsymbol{x}_j^{OUT} . \boldsymbol{x}_{j+1}^{IN} & \boldsymbol{y}_j^{OUT} . \boldsymbol{x}_{j+1}^{IN} \\ \boldsymbol{x}_j^{OUT} . \boldsymbol{y}_{j+1}^{IN} & \boldsymbol{y}_j^{OUT} . \boldsymbol{y}_{j+1}^{IN} \end{pmatrix}$$

We can compute the angle of incidence at mirror $j$ according to

$$\cos 2\theta_j = \boldsymbol{m}_{j,j-1} . \boldsymbol{m}_{j,j+1}.$$

In a ray-matrix basis of the form $\begin{bmatrix} x\ position \\ y\ position \\ x\ slope \\ y\ slope \end{bmatrix}$, the propagation operator to move (half the distance) between mirror *j-1* to mirror $j$ may be written independently for **x** and **y** axes as

$$\mathbf{PROP}_\mathrm{j} = \begin{pmatrix} 1 & 0 & |\boldsymbol{M}_{j-1,j}|/2 & 0 \\ 0 & 1 & 0 & |\boldsymbol{M}_{j-1,j}|/2 \\ 0 & 0 & 1 & 0 \\ 0 & 0 & 0 & 1 \end{pmatrix}.$$

The basis transformation from the coordinates from after mirror $j$ to the coordinates before mirror $j$+1 is

$$\mathbf{ROT}_j = \begin{bmatrix} \mathbf{R}_j & 0 \\ 0 & \mathbf{R}_j \end{bmatrix}.$$

The matrix for reflection off of mirror $j$, including astigmatism from non-normal reflection, is

$$\mathbf{MIRROR}_j = \begin{pmatrix} 1 & 0 & 0 & 0 \\ 0 & 1 & 0 & 0 \\ \frac{-2}{ROC_j} \cos\theta_j & 0 & 1 & 0 \\ 0 & \frac{-2}{ROC_j} \frac{1}{\cos\theta_j} & 0 & 1 \end{pmatrix}.$$

Referenced to the plane midway between the $j$ = 1 and $j$ = $n$ mirror, the round-trip 4x4 ABCD matrix may now be written as

$$\mathbf{M}_{\mathrm{rt}} = \prod_{j=1}^{n} \mathbf{PROP}_j \cdot \mathbf{ROT}_j \cdot \mathbf{MIRROR}_j \cdot \mathbf{PROP}_j$$

To compute the mode spectrum, we make use of techniques developed in[44]. The eigenvalues and corresponding eigenvectors of $\mathbf{M}_{\mathrm{rt}}$ are computed numerically, and labeled $\epsilon_k$ and $V_k$, respectively. When the resonator is stable, all of the eigenvalues have magnitude unity, and come in conjugate pairs. We will choose these pairs to be k=1,3 and k=2,4 so that we can analyze k=1,2 as the two independent eigenmodes.

The transverse mode spacings are $\nu_k \equiv \frac{c}{L_{rt}} \frac{\log \epsilon_k}{2\pi i}$, where $c$ is the speed of light, and $L_{rt} = \sum_j |\boldsymbol{M}_{j,j+1}|$ is the round-trip resonator length. To compute the $TEM_{00}$ mode wavefunction and corresponding raising operators, we require a few more definitions

$$\mathbf{G} = \begin{pmatrix} 0 & 0 & 1 & 0 \\ 0 & 0 & 0 & 1 \\ -1 & 0 & 0 & 0 \\ 0 & -1 & 0 & 0 \end{pmatrix}$$

$$N_k = V_k^{\dagger} \cdot \boldsymbol{G} \cdot V_k, \text{ and}$$

$$\tilde{V}_k = V_k / \sqrt{N_k/2}.$$

Finally, we define the 2x2 matrices **B** and **K** as

$$\begin{pmatrix} \mathbf{B} \\ \boldsymbol{i}\,\mathbf{K} \end{pmatrix} \equiv (N_1 \quad N_2).$$

The $TEM_{00}$ mode may be written, up to a normalization constant (with $\boldsymbol{r} \equiv \begin{pmatrix} x \\ y \end{pmatrix}$) as

$$\psi_{00}(\boldsymbol{r}) \propto e^{-\frac{\pi}{\lambda}\boldsymbol{r}^{\intercal} \cdot \mathbf{B}^{-1} \cdot \mathbf{K} \cdot \boldsymbol{r}}.$$

In the plane midway between mirrors 1 and $n$, the mode waists along the two (orthogonal) principal axes are thus given in terms eigenvalues $d_i$ of the inverse complex beam parameter matrix $Q^{-1} \equiv i\,\mathbf{B}^{-1} \cdot \mathbf{K}$ by

$$w_k = \sqrt{\frac{\lambda}{-\pi\, Im(d_i)}},$$

where $\lambda$ is the wavelength of the light propagating in the resonator. Figure S2a plots the waist size of our resonator as the on axis length is varied while keeping the opening half angle fixed at 16 degrees. We see a broad stable region with waist sizes on the order of 40 microns. Figure S2b explores the transverse mode splittings. We find the resonator parameters that create the desired degeneracy (Fig. S2c) by finding resonator parameters where three times a transverse mode splitting equals one free spectral range of the resonator. The higher order transverse modes may be generated using raising operators, given by

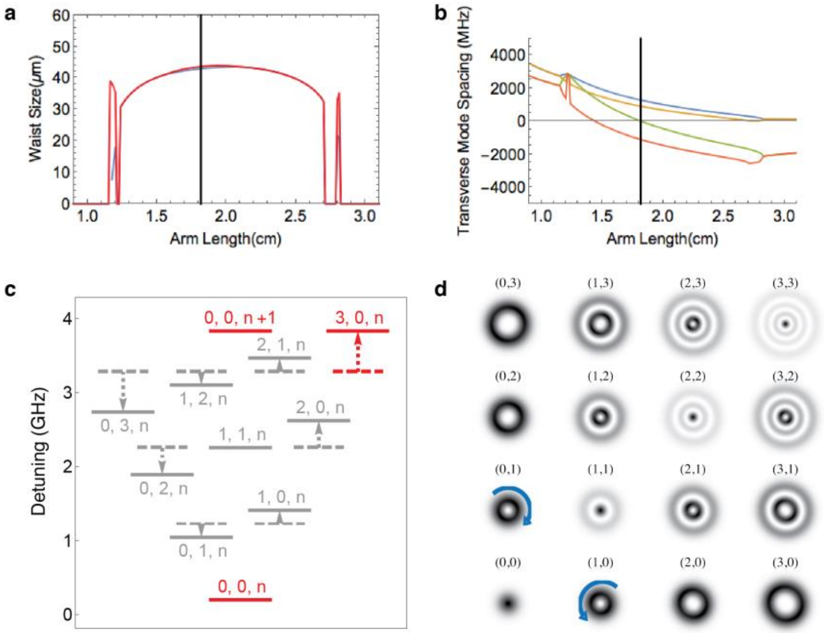


**Figure S2. a,** *Ab initio* mode calculations provide the waist sizes of a stretched tetrahedral non-planar resonator with an opening half-angle of 16 degrees as the axis length is varied. A region of stability is observed between on axis lengths $L_a$ = 1.2 cm and $L_a$ = 2.7 cm; as indicated by the vertical bar the experimental resonator has an on axis length $L_a$ = 1.816 cm corresponding to waist sizes $w_0$ = 43 μm. Residual astigmatism causes the two transverse waist sizes to be unequal. **b,** For the same resonator configurations as in **a**, the transverse mode spacings are plotted (blue and yellow) along with three times the transverse mode spacings minus one free spectral range (green and red). We see that the latter both cross zero within the region of stability. We operate where the green curve crosses zero frequency. **c,** The energy spectrum of the resonator (solid lines) is that of a harmonic oscillator in a magnetic field. The magnetic field splits (gray arrows) right- and left-handed modes that would be degenerate without a magnetic field, i.e. of *planar* resonator of identical parameters (dashed lines). The modes are labeled by two transverse mode numbers ($\alpha, \beta$) and the longitudinal mode number $n$. To create a photonic Landau level on a cone, our resonator is engineered so that each (0,0) mode is degenerate with the ($3p$,0) modes from $p$ free spectral ranges away. By confining our attention to a particular transverse plane and recognizing a separation of energy scales, we can ignore the longitudinal degree of freedom. **d,** The first few transverse modes of the experimental resonator are plotted using the *ab initio* calculations. Each profile is labeled by mode numbers ($\alpha$, $\beta$), corresponding to $\alpha$ units of positive angular momentum and $\beta$ units of negative angular momentum. The modes are quasi-Laguerre-Gaussian with small corrections from residual astigmatism. The total angular momentum of resonator photons is given by $l = \alpha - \beta$; when $\beta = 0$, we label modes only by their angular momentum $l$. Additionally, these modes have phase winding $e^{il\phi}$, as represented by the blue arrows. Our photonic lowest Landau level consists of the $l$ = 0, 3, 6, … modes, which appear as rings of increasing size. Any superposition of these modes will necessarily display threefold symmetry.

$$a_k^\dagger \equiv -i\sqrt{\frac{\pi}{\lambda}}\tilde{V}_k^\dagger \cdot \mathbf{G} \cdot \begin{pmatrix} x \\ y \\ \partial_x \\ \partial_y \end{pmatrix}.$$

Therefore, we calculate any transverse mode of the resonator as

$$\psi_{\alpha\beta}(\boldsymbol{r}) = \frac{1}{\sqrt{\alpha!\beta!}} {a_1^\dagger}^\alpha {a_2^\dagger}^\beta \psi_{00}(\boldsymbol{r}).$$

Figure S2d plots the first few transverse modes of our resonator calculated using this *ab initio* technique. The raising operator description of the resonator modes emphasizes the simple double-ladder pattern in the resonator spectrum: $a_1^\dagger$ adds one energy quantum and one unit of

positive angular momentum, and $a_2^\dagger$ adds another energy quantum and one unit of negative angular momentum. The ($\alpha$, $\beta$) modes carry $l = \alpha - \beta$ units of angular momentum. For our resonator, the modes resemble slightly deformed Laguerre-Gauss $LG_{\alpha\beta}$ modes, where the deformation arises due to residual astigmatism.

**5. Understanding twisted resonators in the ray picture** A twisted resonator composed of planar mirrors exhibits only round-trip image rotation, about the resonator axis, by small angle Θ[28], thus making each plane transverse to the resonator axis behave as a stroboscopically evolving non-inertial reference frame with Coriolis- and centrifugal- forces. To make the resonator stable, we must add mirror curvature, which provide confinement that competes with the centrifugal force. Exploring the Poincaré hit-patterns that result from plotting out round-trip ray trajectories is instructive for understanding the interplay of harmonic trapping and rotation that gives rise to both the lowest Landau level physics and the degeneracy that gives rise to Landau levels on a cone.

In Figure S3a, we display a typical round-trip ray trajectory (henceforth "hit-pattern") in a twisted optical resonator with planar mirrors: the hit-location simply orbits the resonator axis. The round-trip rotation angle Θ determines to the coarseness of the sampling of this circular orbit—we plot a rotation angle $\Theta \sim 2\pi/60$.

In Figure S3b, we display what happens when the mirrors induce harmonic trapping with a frequency equal to the rotation frequency – when the real-space rotation per round trip Θ induced by the resonator twist is equal to the phase-space rotation per round trip ϕ induced by mirror curvature. Under these conditions we are left with cyclotron orbits, corresponding to Landau level physics in the wave/quantum regime. These cyclotron orbits are *not* centered on the resonator axis, as a particle in *only* a magnetic field has no preferred axis (the gauge employed to compute dynamics may have a preferred axis, but this is a non-physical computational tool); the cyclotron orbits circulate around guiding centers $\boldsymbol{r}_c \equiv \boldsymbol{r}_0 - \frac{\hat{\boldsymbol{z}} \times \boldsymbol{p}_0}{qB}$, where $\boldsymbol{r}_0$ and $\boldsymbol{p}_0$ are the initial ray position and (canonically conjugate) momentum, respectively. In our case the conjugate momentum has a physical significance: it is the ray slope relative to the resonator axis, times the total photon momentum $\hbar$k.

If the harmonic confinement is not perfectly compensated, as in Figure S3c, the system again has a preferred axis given by the center of the trap, and there is a slow magnetron precession of the cyclotron orbit about this axis.

Thus far we have considered the situation of small real- and phase-space rotations per resonator round-trip, $\Theta, \phi \ll 1$; this seemed appropriate, as we wanted to coarse-grain away the fact that our rays are repeatedly traversing the resonator structure. One can achieve such coarse graining in other limits, however: in Figure S3d we consider the situation where the rays return near their initial locations after three round-trips: $|\theta| + |\phi| \approx \frac{2\pi}{3}$; alternatively, this situation may be viewed as setting the magnetron frequency to one third of the round-trip (axial) frequency. Under such conditions, we get three copies of the cyclotron dynamics—three copies of a photon in a magnetic field, rotated by 120 degrees with respect to one another. The coarseness of the coverage of the cyclotron orbit (and hence cyclotron frequency) is now determined by how

commensurate either $\Theta$ or $\phi$ is with $2\pi$. This is the configuration that we employ in the present experimental work. Note that neither Θ nor ϕ is individually constrained to be $\sim\frac{2\pi}{3}$; only their sum (or difference) is constrained.

**6. Extracting Hamiltonian parameters for the twisted resonator** In order to extract, from the ABCD matrix, the parameters of our longitudinally coarse-grained dynamics, we employ techniques developed in a theoretical work on engineering photonic Floquet Hamiltonians[28]. We summarize the key results below:

1. For a system with ABCD matrix **M** describing round-trip propagation through the resonator, the effective Floquet Hamiltonian may be written:
$$H = \frac{c}{L_{rt}}[\frac{1}{2}(\boldsymbol{p}^{\intercal} \quad -\boldsymbol{x}^{\intercal})(\log \boldsymbol{\beta}\mathbf{M}\boldsymbol{\beta}^{-1})\begin{pmatrix}\boldsymbol{x}\\ \boldsymbol{p}\end{pmatrix}]$$
Here $\boldsymbol{\beta} \equiv \begin{pmatrix}1 & 0\\ 0 & \hbar k\end{pmatrix}$ converts between ray slope and ray transverse momentum, which is the quantity which is canonically conjugate to ray position. $L_{rt}$ is the round-trip propagation distance through the resonator.
2. Because our resonator requires $s$ = 3 round trips through the resonator to generate a low-energy manifold, the above result is employed with $\boldsymbol{M} \to \boldsymbol{M}^s$, $L_{rt} \to s\, L_{rt}$. This means that all frequencies are defined only modulo a third of the resonator free spectral range.
3. This Hamiltonian may then be completely decomposed according to:
$H = \frac{1}{2}(\boldsymbol{p} - \beta_k\boldsymbol{\sigma}^k \cdot \boldsymbol{x})^{\intercal}\boldsymbol{m}_{eff}^{-1}(\boldsymbol{p} - \beta_k\boldsymbol{\sigma}^k \cdot \boldsymbol{x}) + \frac{1}{2}\boldsymbol{x}^{\intercal}\boldsymbol{\omega}_{trap}^{\intercal}\boldsymbol{m}_{eff}^{-1}\boldsymbol{\omega}_{trap}\boldsymbol{x}$, where
$$\boldsymbol{m}_{eff}^{-1} = \frac{1}{m}R_{\theta_m}.\begin{pmatrix}\frac{1}{1+\epsilon_m} & 0\\ 0 & \frac{1}{1-\epsilon_m}\end{pmatrix}.R_{-\theta_m},$$
$$\boldsymbol{\omega}_{trap} \equiv \omega \cdot R_{\theta_t}.\begin{pmatrix}1+\epsilon_t & 0\\ 0 & 1-\epsilon_t\end{pmatrix}.R_{-\theta_t},$$
$$\boldsymbol{\sigma}^{\boldsymbol{k}} = [\boldsymbol{I}, \boldsymbol{\sigma}^x, \boldsymbol{\sigma}^y, \boldsymbol{\sigma}^z],$$
$$\beta_k = \left[\delta, \Delta_\times, \frac{iB_z}{2}, \Delta_+\right],$$
$$R_\phi \equiv \begin{pmatrix}\cos\phi & \sin\phi\\ -\sin\phi & \cos\phi\end{pmatrix},$$

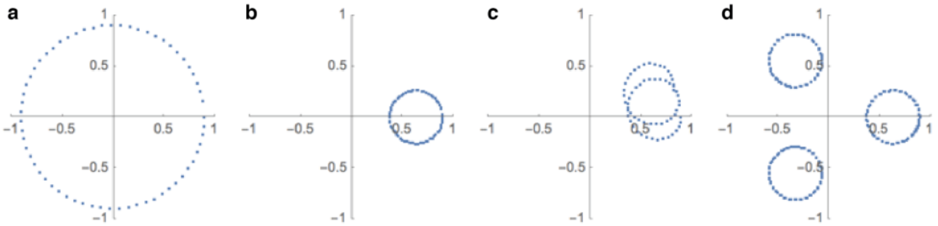


**Figure S3 | Round-trip hit pattern for rays in various twisted resonator configurations. a,** For a twisted resonator without any harmonic confinement (mirror curvature), rays orbit the resonator axis. **b,** When the harmonic confinement precisely cancels the twist-induced centrifugal anticonfinement, closed cyclotron orbits result. **c,** A small amount of residual (anti)confinement produces a slow magnetron precession of the cyclotron orbit. **d,** When this magnetron precession occurs at one third of the resonator round-trip frequency, we return to the zero-confinement configuration, with three identical copies oriented at 120 degrees from one another, corresponding to a cone such as in our system.

and the Pauli matrices operate on the real-space vector $\boldsymbol{x}$.

This prescription enables us to extract the photon mass, residual trapping and effective magnetic field. It also allows us to determine the extent to which mirror astigmatism produces tensor mass, trap astigmatism, as well as scalar and tensor defocus; the last of these (defocus) may be gauged away.

Applying this technique to our resonator structure, for the parameters given by our anticipated degeneracy condition (when the round-trip Gouy phase for one of the eigenmodes is $2\pi/3$) yields the following physical parameters:

$$m \approx 1.06 \times 10^{-4} m_e, \epsilon_m \approx 1.8 \times 10^{-2}, \theta_m \approx -47.1^o$$
$$\omega_{trap} \approx 2\pi \times 180 \text{ Hz}, \epsilon_t \approx -4.2 \times 10^{-2}, \theta_t \approx -42.8^o$$
$$\omega_{cyc} \equiv \frac{eB}{m} \approx 2\pi \times 370 \text{ MHz}$$
$$l_B \equiv \sqrt{\frac{\hbar}{qB}} \approx 22\ \mu\text{m}$$

The key point is that while trap astigmatism persists all the way to the degeneracy point, the trap frequency itself goes to zero (and indeed changes sign), meaning that there is not residual astigmatism that persists at "degeneracy" to destroy the Landau levels.

We employed $\mathbf{M}^3$ for the Floquet formalism since it is only on three round trips that rays return to the same cyclotron orbit in which they started (see Fig. S3d), thus intuitively corresponding to a planar geometry. However, creating a single cyclotron orbit without threefold symmetry requires mixing the three flux-threaded cones. This aliases frequencies by one third the free spectral range rather than simply the free spectral range and is further manifested through an increased photon *mass*. The magnetic length is unaffected, as it does not depend upon the photon mass.

Therefore, to compare with experiment, we may have to add a multiple of one third of the free spectral range to the calculated cyclotron frequency. Quantitatively, the calculated $\frac{\nu_{FSR}}{3} \approx 2\pi \times$ 3.824 MHz/3$\approx 2\pi \times 1.274$ GHz, so the predicted bare (unrolled) cyclotron frequency before aliasing is $\omega_{cyc}^{unrolled} = \omega_{cyc} + \frac{2\nu_{FSR}}{3} \approx 2\pi \times 2.178$ GHz, which agrees with the measured cyclotron frequency of $2\pi \times 2.167$ GHz listed in the main text, up to a corrections arising from imperfect knowledge of mirror curvature and geometric uncertainty from machining imperfections.

The aliasing of the cyclotron frequency directly causes an apparent discrepancy between the mass derived from the Floquet theory and that which we experimentally measure. Recalling the expression for the photon mass $m = \frac{4\hbar}{\omega_c w_0^2}$, we can see that the ratio of aliased to actual cyclotron frequencies will give the inverse of the increased to actual photon mass: $\left(\frac{\omega_{cyc}}{\omega_c}\right)^{-1} = \left(\frac{0.370}{2.167}\right)^{-1} =$ 5.86 while $\frac{m_{Floq}}{m_{exp}} = \frac{10.6}{1.84} = 5.8(3)$.

Within a Landau level, the effective harmonic trapping is given by $\frac{1}{2}m\omega^2 r^2 \approx \frac{\omega^2}{\omega_{cyc}}(a_R^\dagger a_R + a_L^\dagger a_L)$, where $a_{R,L}^\dagger$ add a quantum of angular momentum within a Landau level, and promote to the next higher Landau level, respectively. Thus the harmonic trapping induces a splitting between angular momentum states of $\frac{\omega^2}{\omega_{cyc}}$. We find that the harmonic trapping frequency $\omega$ goes as the square root of the axial resonator length defect, so the splitting between states in a nearly degenerate Landau level is linear in the length as observed experimentally in the main text.

**7. More on the Landau level structure of our resonator** By choice of the position of the four resonator mirrors, no matter the initial mode, increasing the first transverse index by three results in another degenerate mode. Therefore, we may label each Landau level by the indices of its 'fundamental' mode, which may take the form $(i, \beta)$ for $i \in \{0,1,2\}$ and $\beta \in \mathbb{Z}^*$, the non-negative integers. For example, the degenerate set consisting of the (1,4); (4,4); (7,4); … modes may be called the (1,4)-Landau level.

Up to normalization, an arbitrary Laguerre Gauss mode may be written in the following form: $LG_{\alpha,\beta}(z = (x+iy)/w_{00}) = \left(\partial_z - \frac{\bar{z}}{4}\right)^\beta z^\alpha \exp\left(-\frac{|z|^2}{4}\right)$. This yields the following equations for the modes:

$LG_{\alpha,\beta} = z^{\alpha-\beta} f_\beta(|z|^2;\alpha) \exp\left(-\frac{|z|^2}{4}\right)$ where the first few radial functions are

$$f_0(|z|^2;\alpha) = 1$$
$$f_1(|z|^2;\alpha) = \alpha - |z|^2$$
$$f_2(|z|^2;\alpha) = \frac{|z|^4}{4} + \alpha(\alpha - 1 - |z|^2)$$
$$f_3(|z|^2;\alpha) = -|z|^6 + \frac{3}{4}\alpha|z|^4 + \alpha(\alpha-1)\left(\alpha - 2 - \frac{3}{2}|z|^2\right)$$
$$f_4(|z|^2;\alpha) = \frac{|z|^8}{16} - \frac{1}{2}\alpha|z|^6 + \frac{3}{2}\alpha(\alpha-1)|z|^4 + \alpha(\alpha-1)(\alpha-2)(\alpha-3-2|z|^2)$$

Our system breaks apart the traditional lowest Landau level, which includes all angular momentum states, into three separate sets. These sets are {(*0,0*); (*3,0*); (*6,0*); …}, {(*1,0*); (*4,0*); (*7,0*); …}, and {(*2,0*); (*5,0*); (*8,0*); …}. In our system, each of these sets is itself the lowest Landau level on one of three *cones*, which may be labeled by an integer $c = 0$, $1$, or $2$, respectively.

First, we show that the {(*0,0*); (*3,0*); (*6,0*); …} set, or the (0,0)-Landau level, may be said to be the lowest Landau level on a cone. This arises from a symmetry of these modes, namely that $\psi(\theta + 2\pi/3) = \psi(\theta)$. As depicted in Fig. 1d, this symmetry allows the identification of two rays from the center separated by an angle $2\pi/3$. The full plane is then three identical images of this cone. In the reduced space of this cone, the quantum of angular momentum is naturally three times larger than in the full plane, so the (0,0)-Landau level contains all allowed angular momentum states within this cone.

The other two sets are similarly lowest Landau level on two other cones. The symmetry for these is more complicated: $\psi(\theta + 2\pi/3) = e^{2\pi ic/3}\psi(\theta)$, where $c$ identifies on which cone the modes live.

We may then apply a different local gauge transformation to the modes of each set depending on $c$. If we write $\varphi(\theta) = \psi(\theta)e^{-ic\theta}$, then we recover the symmetry of a cone for all $c$, namely that $\varphi(\theta + 2\pi/3) = \varphi(\theta)$. Therefore, we justify the claim that each of the sets is a lowest Landau level on a different cone by appealing to a symmetry condition of the modes of each set *after applying a different local gauge transformation for each set*. The extra phase factor in the symmetry condition has additional effects, which we will explore later in the section titled "The local density of states and flux threaded cones".

One may then ask what the first excited Landau level looks like on each cone. The (0,0)-Landau level clearly satisfies $\psi(\theta + 2\pi/3) = \psi(\theta)$, as $z^\alpha = r^\alpha e^{i\alpha\theta}$ and $\alpha$ is divisible by 3. The next lowest Landau level that satisfies the periodicity condition is the (1,1)-Landau level. In general, excitation to a higher Landau level within a given cone is produced by incrementing both $\alpha$ and $\beta$ by one. In other words, the ladder of Landau levels on the $c^{th}$ cone are the ($\beta$+$c$ mod 3, $\beta$)-Landau levels. Therefore, the cyclotron frequency, which is simply the frequency spacing between Landau levels, is the frequency spacing between the (0,0) and (1,1) modes. $\omega_c$ = 2.1671(2) GHz.

To summarize, at degeneracy every mode of the resonator resides in a Landau level, and we can sort any mode ($\alpha$, $\beta$) into the ($\alpha$ mod 3, $\beta$)-Landau level residing on the $c$ = ($\alpha$ – $\beta$) mod 3 cone. Figure S4 sorts many low-lying modes into the correct cone and Landau level according to this rule.

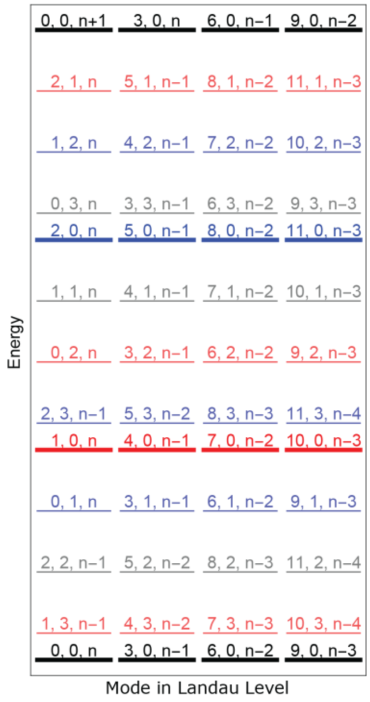


**Figure S4.** Low lying modes are sorted into their appropriate cone and Landau level. Modes are labeled by their two transverse indices and then their longitudinal index. Levels colored in black, red, or blue correspond to the cones with $c$ = 0, 1, or 2 respectively. The bold sets are the lowest Landau levels on each cone.

For future interacting physics utilizing our resonator design, it is essential that no Landau levels reside too close the desired (0,0)-Landau level. Since there are a (countably) infinite number of Landau levels precessing (in general) incommensurately through a free spectral range, there will be a Landau level arbitrarily close to any other. The (1,3)-Landau level is 123 MHz from the (0,0)-Landau level. The (2,10)-Landau level jumps an order of magnitude closer in frequency to 15.2 MHz separated, and the (2,83)-Landau level jumps another order of magnitude closer at 0.71 MHz separated. Disorder much smaller than the mode size couples modes without regard to their phase profiles, so only intensity non-overlap prevents such disorder from coupling nearby Landau levels. Larger disorder also couples levels, but additional phase non-overlap causes suppression. This results in ~20 protected modes in the (0,0)-Landau level.

The choice of degeneracy parameter $s = 3$ was largely arbitrary in this work, and this discussion easily generalizes. While a degeneracy parameter $s = 1$, or 2 is difficult to realize as we would need to remove astigmatism through compensatory astigmatic supermirrors, higher order degeneracies $s > 3$ are certainly possible.

**8. Invariance under magnetic translations of lowest Landau level modes in the Laguerre-Gauss basis** The wavefunctions of the lowest Landau level may be represented in the convenient form $\psi_l \propto z^l e^{-z\bar{z}}$, where $z \equiv (x + i\,y)/w_0$ is a *complex* representation of the 2D particle position, with $w_0$ being the (0,0) mode's $1/e^2$ intensity radius. These modes are also the Laguerre-Gauss solutions to the paraxial wave equation.[41]

It is not immediately obvious how the $\psi_l$ translate, as each $\psi_l$ seems to have a well-defined center located at $z$=0. Here we show that in fact any of these levels arbitrarily translated in the x-y plane may be represented, up to an additional phase, by a sum over the states of the lowest Landau level. This phase reflects that the system is invariant under magnetic translations, not simple translations.

Suppose that the state we would like to represent is a $\psi_\alpha$ centered at ($x_0$,$y_0$). We first define $z_0 \equiv (x_0 + iy_0)/w_0$; we are inclined to see if $\psi'_\alpha = (z - z_0)^l e^{-|z-z_0|^2}$ may be represented as a superposition of the $\psi_l$, but the correct wavefunction differs by a spatially varying phase: $\phi = (z - z_0)^\alpha e^{-|z-z_0|^2} e^{z\bar{z}_0 - \bar{z}z_0}$, where the exponent in the second term is imaginary by construction. We now expand out the first exponential, re-arrange terms, and Taylor expand in powers of z:

$$\phi = (z - z_0)^\alpha e^{-(z\bar{z} + z_0\bar{z}_0 - z\bar{z}_0 - \bar{z}z_0)} e^{z\bar{z}_0 - \bar{z}z_0} = (z - z_0)^\alpha e^{-|z|^2 - |z_0|^2} e^{2z\bar{z}_0}$$

$$= \sum_{k=0}^{\alpha} \binom{\alpha}{k} z^k (-z_0)^{\alpha-k} e^{-|z|^2 - |z_0|^2} \sum_{n=0}^{\infty} \frac{(2\bar{z}_0)^n}{n!} z^n$$

$$= e^{-|z|^2 - |z_0|^2} \sum_{n=0}^{\infty} \sum_{k=0}^{\alpha} \binom{\alpha}{k} (-z_0)^{\alpha-k} \frac{(2\bar{z}_0)^n}{n!} z^{n+k}$$

$$= \sum_{l=0}^{\infty} \left( e^{-|z_0|^2} \sum_{k=0}^{\min(l,\alpha)} \binom{\alpha}{k} (-z_0)^{\alpha-k} \frac{(2\bar{z}_0)^{l-k}}{(l-k)!} \right) z^l e^{-|z|^2}$$

The final expression is clearly a sum over lowest Landau level wavefunctions, demonstrating the desired magnetic translational invariance. The additional phase required for the translation reflects that the translation operator in a magnetic field is not the simple translation $T = e^{-\frac{i}{\hbar}\hat{\boldsymbol{p}}\cdot\hat{\boldsymbol{r}}}$, but instead is the magnetic translation operator, which takes the form $T = e^{-\frac{i}{\hbar}(\hat{\boldsymbol{p}}+e\hat{\boldsymbol{A}})\cdot\hat{\boldsymbol{r}}}$ in the symmetric gauge. The apparent preferred center of Laguerre-Gauss modes does not imply a preferred center for dynamics; in fact, the dynamics are translationally invariant and the Laguerre-Gauss mode basis is ideal for writing the Laughlin wavefunction of the fractional quantum Hall effect[45].

It is straightforward to extend this to our lowest Landau level consisting of modes $(\alpha, 0)$ with $\alpha = 0, 3, 6, \ldots$ under the requirement that we do not displace a mode alone, but rather create two additional displaced copies rotated to preserve threefold symmetry. That is, we send $z_0 \to z_a = z_0 e^{2\pi i a/3}$ for $a = 0, 1, 2$, and introduce the sum $\sum_{a=0}^{2}$ . Therefore, we wish to show that

$$\phi = \sum_{a=0}^{2} (z - z_a)^{\alpha} e^{-|z-z_a|^2} e^{z\bar{z}_a - \bar{z}z_a} = \sum_{n} C_n \psi_n(z)$$

for some coefficients $C_n$ where the sum over $n$ has been restricted to every third non-negative integer. However, we wish for our displaced mode to have an additional property. As written, $\phi$ can only be expanded on one of the three cones of the system. If we write $n = 3p + c$ and write $\alpha = 3q + d$, then we have the condition that $c = d$, or $(n - \alpha) \bmod 3 = 0$. In fact we can write a displaced version of $\psi_l$ (with copies to preserve 3-fold symmetry) as a sum for any $c \in \{0, 1, 2\}$. That is, any displaced mode can be expressed as a sum of modes on any individual cone. Therefore we consider mode profiles of the form

$$\phi = \sum_{a=0}^{2} (z - z_a)^{\alpha} e^{-|z-z_a|^2} e^{z\bar{z}_a - \bar{z}z_a} e^{\frac{2\pi i a b}{3}}$$

where $b \in \{0, 1, 2\}$ may be chosen so that the mode is on the $c^{th}$ cone. We perform Taylor expansions as before, so that

$$\phi = \sum_{n=0}^{\infty} e^{-|z_0|^2} \sum_{a=0}^{2} e^{\frac{2\pi i a}{3}(\alpha - n + b)} \left( \sum_{k=0}^{\min(n,\alpha)} \binom{\alpha}{k} (-z_0)^{\alpha-k} \frac{(2\bar{z}_0)^{n-k}}{(n-k)!} \right) z^n e^{-|z|^2}$$

Now, the sum over $a$ yields 3 if $(n - \alpha) \bmod 3 = b$ and 0 otherwise. This crucial condition, relating $b$, $c$, and $d$ as $b = (c - d) \bmod 3$, allows for the initial choice of $b$ given the displaced mode on the desired cone. To state the final result,

$$\phi = \sum_{p=0}^{\infty} C(p, \alpha, c, z_0)\, z^{3p+c} e^{-|z|^2}$$

which shows that $\phi$ may be written as a sum of modes in the lowest Landau level on the $c^{th}$ cone. As mentioned before, a local gauge transformation $e^{-ic\theta}$ may be applied to make the wavefunction continuous. This result is useful for mathematically describing the mode profiles needed to create displaced versions of angular momentum states about the origin. More important is the recognition that the displaced angular momentum state may have any integer value of angular momentum, even though it is on a cone that supports only every third state of angular momentum about the cone apex. As long as the displacement is large enough that the mode profile does not overlap with the cone apex, these new displaced angular momentum states will not interfere with themselves and have profiles similar to angular momentum states in flat

space. This means that future investigations need not be limited to Landau levels with only every third angular momentum states, but instead may use Landau levels with every angular momentum state where the angular momentum is measured about a suitably displaced point.

**9. The form of the N-particle bosonic Laughlin state on a cone** On a plane, the bosonic Laughlin wavefunction takes the celebrated form[45]:

$$\Psi_L \propto e^{-\sum_k |z_k|^2} \prod_{i<j} \left(z_i - z_j\right)^2$$

This wavefunction has a second-order zero whenever two particles are in the same location, thereby minimizing the interaction energy; it is made up entirely of single-particle states within the planar lowest Landau level $\varphi_l = z^l e^{-z\bar{z}}$.

One might naturally ask, 'How can we make a Laughlin state in our reduced Hilbert space where we are only allowed every third angular momentum state $\varphi_{3l} = z^{3l} e^{-z\bar{z}}$?'

Physically speaking, a cone looks like flat space away from its tip, with curvature only at the tip itself. Consequently, a Laughlin puddle that neither encircles nor overlaps the cone tip will behave as though it inhabits a plane. On the other hand, a Laughlin puddle that touches or encircles the cone tip is a different story: its *physical form* should be changed due to the Wen-Zee coupling to manifold curvature. We treat these two cases separately.

The translation operator in flat space is $\prod_k e^{z_0(\bar{z}_k - \partial_{z_k})}$. So, the translated Laughlin wavefunction is

$$\begin{aligned}
\Psi_L^{Tr.} &= \prod_k e^{z_0(\bar{z}_k - \partial_{z_k})} \prod_{i<j} \left(z_i - z_j\right)^2 e^{-\sum_p |z_p|^2} \\
&= \prod_k e^{z_0 \bar{z}_k} e^{-z_0 \partial_{z_k}} \prod_{i<j} \left(z_i - z_j\right)^2 e^{-\sum_p |z_p|^2} \\
&= \prod_k e^{z_0 \bar{z}_k} \prod_{i<j} \left(z_i - z_j\right)^2 e^{-\sum_p |z_p - z_0|^2} \\
&= e^{-N|z_0|^2} \prod_{i<j} \left(z_i - z_j\right)^2 e^{-\sum_p |z_p|^2} e^{-\sum_p z_p \bar{z}_0} \\
&= \Psi_L e^{-N|z_0|^2} e^{-\sum_p z_p \bar{z}_0}
\end{aligned}$$

This is the original Laughlin state times an irrelevant normalization factor and an exponential gauge factor. While this changes the form of the wavefunction, it does not affect the order of the zero as two particles approach each other; it leaves the state in the lowest Landau level; and it does not change quasi-hole statistics.

*Away from the Cone Tip*

Away from the cone tip, space is flat, so we should expect that the discussion above implies that a regular Laughlin state (up to the additional exponential factors) is supported. The only question is whether this state lives within the lowest Landau level on the cone.

We write the Jastrow factor in the $N$-particle Laughlin wavefunction as a polynomial (with coefficients $J$) on single-particle wavefunctions:

$$\Psi_L \propto e^{-\sum_k |z_k|^2} \prod_{i<j} (z_i - z_j)^2 = e^{-\sum_k |z_k|^2} \sum_{\{a_1,\dots,a_N\}} \left( J_{a_1,\dots,a_N} \prod_{p=1}^{N} z_p^{a_p} \right)$$
$$= \sum_{\{a_1,\dots,a_N\}} \left( J_{a_1,\dots,a_N} \prod_{p=1}^{N} \psi_{l=a_p}(z_p) \right)$$

where the sum is taken over all possible sets $\{a_1, \dots, a_N\}$ under the requirement that $\sum_{p=1}^{N} a_p = L$ where $L = N(N-1)$ is the total angular momentum of the Laughlin state. It is interesting to note that the Jastrow factor is a Jack polynomial, $J_{101010\dots}^{-2}(z_1, z_2, \dots, z_N)$, the decomposition of which in terms of monomials is known[46]. The partition defining the Jack polynomial is the state in the orbital occupation basis that lists the number of particles in the $l^{\text{th}}$ angular momentum state. Thus, this decomposition is the conversion between the second quantized orbital occupation basis into the first quantized particle state basis that lists the angular momentum of each identifiable particle.

Using the results of section 8, the single-particle wavefunction with angular momentum $l$ may be translated by $z_0$ while remaining within the lowest Landau level. Applying this result to the many-body Laughlin wavefunction yields:

$$\Psi_L^{Tr.,Cone}(z_0) = \sum_{\{a_1,\dots,a_N\}} \left( J_{a_1,\dots,a_N} \prod_{p} \left( \sum_{q} C(q, l_p, c, z_0) z_p^{3q+c} e^{-|z_p|^2} \right) \right)$$

This explicitly writes the threefold symmetric translated Laughlin state as a sum of products of lowest Landau level states on the cone. The idea, then, is that this Laughlin wavefunction looks like three copies of a Laughlin puddle, since, so long these copies don't touch one another (*as long as they don't encircle the cone tip*), there will be no self-interactions/interference, and the short range behavior (order of zeroes, etc.) will be identical to the standard planar Laughlin state. It is important to note that we *do not* have three independent Laughlin puddles; the copies have no dynamical degrees of freedom, just as a person's reflection in a mirror is entirely constrained by the person's motion.

*At the Cone Tip*

The story at the cone tip is much more complex, as the Laughlin puddle couples to the manifold curvature directly, and is thereby deformed. Taking the limit $\lim_{z_0 \to 0} \Psi_L^{Tr.,Cone}(z_0) = 0$; the three copies of the planar Laughlin puddle destructively interfere with one another. We must then come up with an ad-hoc wavefunction:

We have not explored it thoroughly, but a three-fold symmetric lowest Landau level wavefunction, centered on the cone tip, with no contact interaction, is:

$$\Psi_L^{cone\ tip} \propto e^{-\sum_k |z_k|^2} \prod_{i<j} (z_i^3 - z_j^3)^2$$

which may be rewritten as

$$\Psi_L^{cone\ tip} \propto \left[ e^{-\sum_k |z_k|^2} \prod_{i<j} \left(z_i - z_j\right)^2 \right] \prod_{p<q} \left(z_p^2 + z_p z_q + z_q^2\right)^2$$

This wavefunction bears similarities to the Laughlin wavefunction, but with an additional post-factor. Because this post-factor is a symmetric polynomial of $z$, it does not influence the order of the zero when two particles approach each other or any other anti-symmetry property. Instead, it changes the angular momentum of the 'center of mass' of the particle distribution, from $L_{CM} = 0$ for the canonical Laughlin state to $L_{CM} = 2N(N-1)$ for the $N$ particle Laughlin state around the cone tip.

*Experimental considerations*

The rich physics of fractional quantum Hall states in curved space is almost completely unexplored experimentally, so it will be fascinating to attempt to build Laughlin states both at and away from the cone tip, and compare their properties. We have explored the feasibility of creating these states in an apparatus that incorporates the nonplanar resonator of the present work into the simultaneously developed cavity Rydberg EIT system that is described in Jia, et al.[47], which will provide the necessary strong photon-photon interactions.

The present work demonstrates that a resonator may support photonic Landau levels at least twenty states accessible. The primary challenge, then, in creating photonic Laughlin puddles is in generating sufficiently strong photon-photon interactions. In planning to use cavity Rydberg EIT, we need to ensure that several conditions are met:

1. The EIT window must be large compared to the lowest Landau level width.
2. Photon-photon interactions must be strong enough that the Laughlin manybody gap is large compared to e.g. the Laughlin state linewidth.

These conditions may be met with experimentally reasonable parameters. While many aspects of this are beyond the scope of the present work, it is important to mention that the mode waist size of the resonator is an important parameter that we will use to meet these requirements: the effective interactions increase as the mode waist is made smaller. However, as the photons are more tightly confined, their interactions, which are effectively finite range, look less like contact interacts, perturbing the form of the Laughlin state. We plan to move from a 43 μm waist to a ~ 20 μm waist, as this will give rise to a substantial increase in interaction strength, while preserving contact-like interactions. Below, we estimate the many-body gap to give a sense for the size of the Laughlin states that can ultimately be attained using Rydberg EIT, and we find that gaps are large enough to accommodate a few tens of polaritons. We also show using numerical simulations that two-polariton Laughlin states can be produced with high fidelity (0.96).

We work in the limit where the Rydberg blockade radius $r_B$ is less than the cavity waist radius $w_0$ so that the polariton-polariton interaction can be approximated as a delta function. The linewidth of an $N$-polariton Laughlin state is then simply $\gamma_L = N\gamma_p$, where $\gamma_p$ is the decay rate of a single polariton.

We estimate the gap for a Laughlin state produced away from the cone tip, where photons reside in a flat-space Landau level. For pure contact interactions, the many-body gap $\Delta_L$ is on the order of the first Haldane pseudopotential $V_0$. For $N = 2$ bosons the gap is[17] $\Delta_L = V_0$, while for large $N$, the gap is[10] $\Delta_L \approx 0.6V_0$. For a contact interaction $V(r) = g_{2D}\delta^{(2)}(r)$ on a plane with s-fold symmetry, the pseudopotential is $V_0 = \frac{g_{2D}}{\pi s w_0^2}$, where s=3 in our case (recall that the magnetic length $l_B = \frac{1}{2}w_0$ and that s=1 on a plane to recover the usual expression). We obtain $g_{2D}$ by integrating the polariton-polariton interaction potential [Sommer, Buchler, Simon arXiv 2015] to obtain $g_{2D} = \frac{-2\pi^2}{3\sqrt{3}}\frac{r_B^2}{\overline{\chi}}$, where $\overline{\chi}$ is the parameter defined in Sommer, *et al.*[16]. Due to photon scattering from the intermediate state in EIT, $\overline{\chi}$ is a complex quantity, leading to a complex many-body gap. The imaginary part of the gap allows the Laughlin state to be selected dissipatively, as the excited states have larger linewidth by an amount given by the size of the imaginary part of the gap.

To enhance the interaction strength, we consider a cavity with a smaller waist $w_0$ = 20 μm, which can also be readily attained. Furthermore, we consider an atomic density of 1 $\mu m^{-3}$, a single-photon detuning of 16 MHz from the intermediate state, and dark state rotation angle of 63°, and excitation to the 95S Rydberg level. We then obtain $|V_0|$= 4.0 MHz, giving $|\Delta_L|$= 2.4 MHz in the large $N$ limit. The linewidth of the rubidium 95S Rydberg level at room temperature is less than 1 kHz[48]; however, the effective linewidth $\gamma_R$ is increased owing to dephasing of the collective Rydberg component of the polaritons, as well as finite laser linewidth. A modest linewidth of $\gamma_R$= 100 kHz, gives a total single-polariton linewidth of $\gamma_p$ = 120 kHz, including loss through the small photonic component of the polariton[47] for a cavity linewidth of $\kappa$ = 200 kHz. In that case Laughlin states of up to $N \sim |\Delta_L|/\gamma_p \sim 20$ polaritons can be resolved. A more optimistic effective Rydberg linewidth of $\gamma_R$= 10 kHz gives a single-polariton linewidth of $\gamma_p$ = 50 kHz for the same cavity linewidth, giving access to Laughlin states of potentially up to 50 polaritons.

To demonstrate one possible preparation method, we numerically simulate driving the cavity with a weak probe beam away from the cone tip using a mode with one unit of angular momentum. In steady state, such a setup is expected to generate a two-photon Laughlin state[16,17]. We simulate the full three-level dynamics for a collection of 35 atoms in the cavity at randomly assigned locations near the mode waist. We restrict to the vicinity of one of the three off-center regions, and rescale the van der Waals coefficient underlying the Rydberg-Rydberg interactions by $\frac{1}{3^3}$ to reproduce the factor of 3 reduction in the effective interaction owing to the three-fold symmetry. Using the parameters given above, and for the more modest 100 kHz effective Rydberg linewidth, we find that photon pairs emitted from the cavity populate the two-photon Laughlin state with a fidelity of 0.96(2).

**10. Comparison to the proposal of Umucalılar and Carusotto** In 2013, Umucalılar and Carusotto proposed a very clever scheme to generate fractional quantum Hall states of light by injecting Laguerre Gauss photons into a two mirror resonator containing a nonlinear optical medium trapped at the mode waist[19]. This method does not rely on a synthetic magnetic field for light; the modes of the lowest Landau level are not degenerate with one another, and are instead degenerate with additional modes outside the Landau level, as the photons live only in a

spherical harmonic trap. The photons are maintained within the states comprising the lowest Landau level by initially injecting them with the proper angular momentum, and conservation of both angular momentum and energy prevents their leaving. The authors show that under these conditions, their approach allows preparation of few-particle Laughlin states and supports the creation and braiding of quasi-hole excitations.

This proposal truly paves the way to creation of fractional quantum Hall states of light, and indeed played a role in inspiring our work, by raising several technical challenges:
(1) Angular momentum is not conserved in realistic resonators due to mirror astigmatism and disorder. These effects scatter the photons out of the lowest Landau level, destroying the Laughlin state.
(2) To date, only narrowband strong optical nonlinearities have been demonstrated and these rely on Rydberg EIT; the proposal does not address the need to fit transverse modes within a narrow bandwidth. To accommodate this while maintaining a small waist size, a potential solution would be to tune the two-mirror resonator to a degeneracy point, e.g. where both Gouy phases are $2\pi/3$. Nevertheless, no matter how the transverse mode spacing between angular momentum modes is made to be small, these modes will each be degenerate with a large number of other modes. This means that problem (1) persists as mirror disorder and polariton interactions will cause scattering between them.

Our approach solves these problems. Using four mirrors, we engineered a resonator with a synthetic magnetic field, thus enabling us to work in a degenerate manifold of only lowest Landau level modes. This means that aberrations and disorder can only induce scattering within the lowest Landau level; operating on a cone suppresses the impact of astigmatism. Furthermore, the demonstrated degeneracy means that the Rydberg EIT window needs only be a few MHz wide, well within the state of the art. As such the remarkable results of Umucalılar and Carusotto, including the spectroscopic preparation of fractional quantum Hall states and quasi-hole braiding, apply directly to our set-up.

**11. Measurable quantities of quantum Hall systems: topological shift and trapped fractional charge** In this section we explain the relation between the local density and quantum Hall transport coefficients. The shortest way to access this relation is through the effective action technique. The effective action $W[A]$ is an extremely compact way to encode linear response functions, i.e. ground state expectation values of density $\rho$, electric current $j_i$ and stress tensor $T_{ij}$. In a gapped system such as quantum Hall state the effective action depends only on external probes, namely the external electromagnetic field and space geometry.

We start with dependence of the density on external magnetic field $B$. The effective action describing electromagnetic response must satisfy two properties: (i) it has to be gauge invariant, this reflects particle number conservation and (ii) it must be "assembled" only from vector potential $A_\mu$, and space and time derivatives $\partial_\mu = (\partial_0, \partial_i)$. The terms with lowest number of derivatives is the so-called Chern-Simons term

$$W[A] = \frac{\nu}{4\pi}\int dt d^2x\, \epsilon^{\mu\nu\rho}A_\mu\partial_\nu A_\rho = \frac{\nu}{4\pi}\int dt d^2x\, \left(\epsilon^{ij}A_i\dot{A}_j + 2A_0 B\right)$$

where $\varepsilon^{\mu\nu\rho}$ and $\varepsilon^{ij}$ are absolutely anti-symmetric tensors with $\varepsilon^{0xy} = 1$ and $\varepsilon^{xy} = 1$. The coefficient $\nu$ is known in the fractional quantum Hall effect as the filling fraction; it determines the Hall conductivity as will become clear shortly. To obtain charge density we differentiate the effective

action with respect to $A_0$

$$\rho = \frac{\partial W}{\partial A_0} = \nu \frac{B}{2\pi}$$

This relation is used to determine the number of background states on a planar manifold. To obtain the $x$-component of the electric current, $j_x$, we differentiate $W$ with respect to $A_x$ to find

$$j_x = \frac{\partial W}{\partial A_x} = \frac{\nu}{2\pi} E_y$$

this is Hall current with Hall conductance $\sigma_H = \nu \frac{e^2}{\hbar}$ (we restored the units). For the integer quantum Hall state with one filled Landau level, the filling factor $\nu$ is one. Since both density and electric current come from the same term in the effective action (namely, the Chern-Simons term) measuring one determines the other.

Next, we wish to introduce non-trivial ambient geometry. We encode the geometry into an object that is called spin connection $\omega_\mu$. This object is directly analogous to vector potential in that its curl gives the (Ricci) curvature

$$\nabla \times A = B \quad and \quad \nabla \times \omega = \frac{1}{2} R$$

The term in the effective action that contains the lowest number of derivatives and depends on both $A$ and $\omega$ is the so-called Wen-Zee term[12]

$$W[A, \omega] = \frac{\nu \bar{s}}{2\pi} \int dt d^2x \, \epsilon^{\mu\nu\rho} A_\mu \partial_\nu \omega_\rho \; = \frac{\nu \bar{s}}{4\pi} \int dt d^2x \, \left( \epsilon^{ij} A_i \dot{\omega}_j + \frac{1}{2} A_0 R + \omega_0 B \right)$$

Now we compute the density again[49]

$$\rho = \nu \frac{B}{2\pi} + \nu \bar{s} \frac{R}{4\pi}$$

This relation is completely general and holds even in any interacting system. The numbers $\nu$ and $\bar{s}$ characterize the topological phase of matter. Generally $\bar{s}$ (called the mean orbital spin) contains extra information about the topological phase of matter. To illustrate this point, we consider how $\nu$ and $\bar{s}$ depend on which Landau level is filled. For all Landau levels, the filling fraction is the same constant (for us, it is one), but $\bar{s} = (2n+1)/2$, where $n$ labels which Landau level is populated with the lowest Landau level corresponding to $n = 0$. In condensed matter systems, it is difficult to create a substantial enough source of curvature to observe a change in density, but in our optical system, it is done with ease.

Measurement of excess state density derived from a local density of states therefore measures the mean orbital spin. The latter allows us to calculate the value of a dissipationless, quantized transport coefficient known as the Hall viscosity, $\eta_H$, which we now describe[30]. Similarly to how the Chern-Simons term encoded Hall conductivity, $\sigma_H$, the Wen-Zee term encodes the Hall viscosity. Formally, it comes from the variation in the last term in the Wen-Zee action. The Hall conductivity is defined from an off-diagonal two-point function of electric currents

$$\langle j_x j_y \rangle = i\omega\sigma_H$$

while the Hall viscosity is defined from an "off-diagonal" two point function of the stress tensor

$$\langle T_{xx} T_{xy} \rangle = i\omega\eta_H$$

Hall viscosity is a non-dissipative transport coefficient that describes transport of momentum transverse to applied shear. It follows from the Wen-Zee action that (in flat space)

$$\eta_H = \frac{\bar{s}}{2}\rho$$

Thus, in order to determine the Hall viscosity in flat space, it is sufficient to measure $\bar{s}$ through a density measurement in curved space.

**12. The local density of states and flux threaded cones** In order to measure the geometry of the manifold for transverse photon dynamics, we look at the local density of states. Because at degeneracy, the density is a series of delta functions in energy, one for each Landau level, we may fix energy at the energy of a Landau level of interest, and treat the local density of states at that energy as a measure solely of the spatial density of states for that Landau level: $\rho(\boldsymbol{z}) = \sum |\psi_n(\boldsymbol{z})|^2$ where the sum is taken over all single particle states in the Landau level of interest. This is easily measured by injecting each single particle state, i.e. each resonator eigenmode, and collecting the transmitted light on a camera. The images are normalized to equal area and then summed, producing Figures 3g-i.

As discussed in the preceding section, the density of electrons in an integer ($\nu = 1$) quantum Hall system in the on a curved manifold is given by,

$$\rho(\boldsymbol{z}) = \frac{1}{2\pi l_B^2} + \bar{s}\frac{R(\boldsymbol{z})}{4\pi}$$

where $l_B = \sqrt{\frac{\hbar}{eB}}$ is the magnetic length, $\bar{s}$ is the mean orbital spin, and $R(\boldsymbol{z})$ is the local curvature of the manifold. The mean orbital spin is predicted to take values $\bar{s} = \frac{n+1}{2}$, where $n$ indexes the Landau levels with the lowest Landau level being $n = 0$. For the $c = 0$ cone, the effective magnetic field is constant everywhere, so $\rho_0 = (2\pi l_B^2)^{-1}$ is a constant. A delta function of curvature at the cone apex provides the only deviation from constant density, and in the lowest Landau level $\bar{s}$ should be one half, so $\delta\rho(\boldsymbol{z}) = \frac{1}{2}\frac{s-1}{s}\delta(\boldsymbol{z})$ where $s = 3$ is the symmetry parameter that defines the cone. By integrating, we therefore expect to find one third of an extra state localized to the tip due to manifold curvature.

We may explore this behavior alternatively by looking at the known mode profiles of the lowest Landau levels. Using the complex representation of the 2D position $z = x + iy$, these modes are given by $\psi_l(z) = \sqrt{\frac{2^{l+1}}{\pi w_0^2 l!}}\left(\frac{z}{w_0}\right)^l e^{-\left|\frac{z}{w_0}\right|^2}$. We then construct the lowest Landau level local density of states on the $c^{th}$ cone as

$$\rho_c = \sum_{n=0}^{\infty} |\psi_{3n+c}|^2$$

As represented in Figure S5, this predicts a threefold increase in state density near the cone tip; the increase is a Gaussian, and is in fact nothing more than the $l = 0$ mode. This matches the prediction from curvature, as the delta function there only suggests an increase localized to around the origin to approximately the magnetic length, and the waist size, $w_0$ is twice the magnetic length. Upon integrating the excess density, we find $\delta N = 1/3$, in agreement with the prediction. However, setting $c$ to 1 or 2 immediately presents a problem, as the local density vanishes at the cone tip. This reflects that the lowest angular momentum states on these cones are $l = 1$ and $l = 2$, respectively, both of which vanish at the origin. Furthermore, when we integrate the excess density we find $\delta N = 0$ and $-1/3$ respectively. We resolve this by looking at the symmetry relation that defines these cones: $\psi(\theta + 2\pi/3) = e^{2\pi i c/3}\psi(\theta)$. The symmetry relations for the $c = 1$ and $c = 2$ cones suggests that there is $-\Phi_0/3$ and $-2\Phi_0/3$ magnetic flux threaded through the tip where $\Phi_0$ is the magnetic flux quantum, as the extra phase factor appears like an

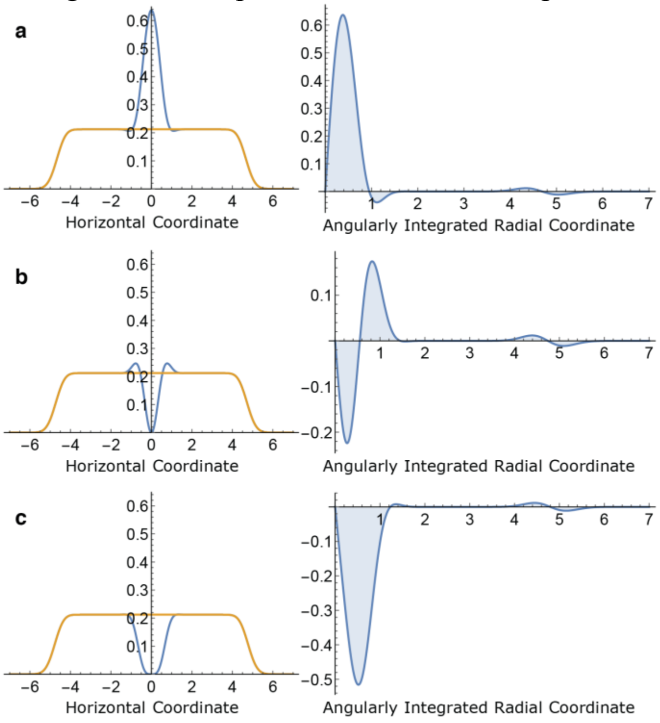


**Figure S5. a,** A slice through the expected local density of states for the $c = 0$ cone shows a threefold increase in density at the apex (blue) above a constant background plateau (yellow). The expected density is presented as a function of radius from the middle after having been integrated in angle. Integrating in radius then provides the total number of excess states (shaded region), which is precisely one third. **b,** the same expected local density of states is shown for the $c = 1$ cone. Although the slice shows a vanishing density at the tip with only a small density increase in a ring around the tip, the angularly integrated expectation shows that these two effects approximately cancel. In fact, the integral is precisely zero. **c,** Finally, the expectation for the $c = 2$ cone is presented, showing a broader decrease near the apex with no counterweighting rise. The integral of the density reveals a deficit of one third of one state.

Aharanov-Bohm phase obtained after encircling the apex. The possibility of extra magnetic flux reflects an inherent ambiguity in the definition of the $2\pi/3$ rotation operator $\hat{R}_3$, which is required to satisfy $(\hat{R}_3)^3 = 1$. Thus three operators $\hat{R}_3$, $e^{2\pi i/3}\,\hat{R}_3$, and $e^{4\pi i/3}\,\hat{R}_3$ are equally good rotation operators, but physically they differ by the presence of an extra 1/3 and 2/3 units of the flux

quantum. Interestingly enough, our system does not pick one of the cases, but realizes all of them leaving it up to us which case to study.

With flux threading, the magnetic field in the equation for state density above is not constant, but rather has a delta function of magnitude $\Phi_c = -2\pi c/3$ at the tip as well. This removes state density from the cone apex, resulting in the following general expectation:

$$\delta\rho(\boldsymbol{z}) = \bar{s}\left(1 - \frac{1 + c/\bar{s}}{s}\right)\delta(\boldsymbol{z})$$

We may perform an integral to find the total state number excess or deficit. Doing so for the lowest Landau level, we predict $\delta N = 1/3$, 0, and $-1/3$ for $s = 3$ and $c = 0$, 1, and 2 respectively, matching the predictions from analytical mode profile integration. This also forms concrete predictions for integer quantum Hall systems in higher Landau levels (using $\bar{s} = (n+1)/2$) as well as on cones of higher degeneracy parameters. As seen in Fig. S5b, the spatial dependence of the density reduction due to flux threading is not the same as the spatial dependence of the density increase due to manifold curvature. This implies that the delta-function description in the equation above is incomplete and points towards the rich interplay between curvature and topology in our system.

We measure the number of excess states on each cone directly from the data without using a fitted curve. We take the local density of states from the first six modes on each cone (Fig. 3g-i). The background plateau value is found as the average of pixel values over an annulus chosen to avoid both the central region and the outer limit. We then sum over pixels within a disk enclosing the central region and subsequently subtract off the average plateau value times the area of the disk. Finally, we convert this quantity to state number by using a conversion factor, which is determined from the integral of the entire image that we know corresponds to six states. We find $\delta N_{c=0} = 0.31(2)$, $\delta N_{c=1} = -0.02(1)$, and $\delta N_{c=2} = -0.35(2)$, where the uncertainty is determined from the choice of the annular background region as well as initial background subtraction.

While we have detected fractional state number excess and depletion at the cone tip, it is worth mentioning that this is unrelated to the fractional charge and fractional statistics of excitations in the *fractional* quantum Hall effect. True excitations in our system correspond to particle-hole pairs each of charge (state number) magnitude one. The fractional state localized to the cone tip is a *defect* in the integer quantum Hall state, which breaks translational invariance and is known as a disclination in solid state physics. The precise value of the state number trapped at the defect is a topological invariant determined by the filling fraction and the discrete rotation symmetry (opening angle of the cone).

Finally, it is worth mentioning another intriguing method for measuring the local density of states. In analogy to scanning tunneling microscopy experiments, we could very tightly focus a Gaussian beam at the resonator waist, and measure the total transmitted optical power as a function of input position. This could map out the local density with a resolution given by the waist size of the incoupled light. One immediate problem presents itself in the requirement that the translated probe must also be tilted to be consistent with magnetic translations; if the tilt is not calibrated correctly, the measured density will be artificially lowered. Additionally, this

method requires implementing high NA optics on the input and output of the resonator, which is technically challenging due to the presence of the resonator mirrors and mounts. Together, these considerations lead us to prefer the implemented method, which provides the same information. With interactions, though, these challenges may be offset by the unique advantages of this method, as it could enable the probing of local excited state density above a spectroscopically prepared fractional quantum Hall ground state.

**13. Twisting light: methods to cause a 2D rotation of light** To create an effective magnetic field for photons, we need to induce a rotation of the transverse light field on each round trip. Such a rotation may in principle be realized using four mirror non-planar resonators, three mirror twisted astigmatic resonators, two mirror spinning astigmatic resonators[50], simple running wave resonators with embedded rotation elements such as dove prisms[51], twisted fiber bundles, or *twisting* or *writhing* waveguides. However, embedded objects cause photon loss incompatible with cavity quantum electrodynamics, astigmatic supermirrors are challenging to manufacture, and waveguides are incompatible with strong interactions. With these considerations, we choose the first approach. We discuss several of these approaches below.

*Four mirror non-planar resonator*

The source of image rotation in our resonator is closely related to the Pancharatnam polarization-rotation under non-planar reflections[52] in non-planar ring-oscillators[53]. The concept is entirely geometrical: any 2-vector is inverted under reflection off of a mirror, and sequential non-parallel inversions are equivalent to a rotation of that 2-vector by the angle between the inversions. A non-planar resonator *generically* provides such non-parallel inversions—both of the image and the polarization—in a closed path where they may occur repeatedly.

*Astigmatic three mirror resonator*

A twisted resonator is most simply realized in a configuration where each of the three mirrors has strongly non-equal radii of curvature, and each is oriented with principal axes rotated by 120 degrees relative to those of the other two (see Fig. S6a). Unfortunately fabricating astigmatic super-mirrors is challenging, so our experiments build upon the four-mirror geometry shown schematically in Fig. 1c.

*Waveguides*

It was recently discovered that knotted-ness of a fluid can be stored in either twist or writhe, and that these two dynamically equilibrate[54]. In this SI we model the transverse motional dynamics of light a single multimode waveguide exhibiting either twist or writhe (see Fig. S6b-c), showing that the guided light experiences an effective magnetic field in both cases. Waveguides are not ideal for entering the fractional quantum Hall regime, however, because achieving photonic interactions requires a strongly interacting mediating medium[1,55] that is difficult to load into even a hollow-core optical fiber[56]. We have discovered that both twisted and writhed configurations may be realized in an ultra-low-loss optical resonator, providing much better access for atom loading.

*Twisting Waveguide*

Light inside of a fiber experiences a paraxial wave equation[22,41]:

$$i\partial_z\psi = \frac{1}{2\mathrm{k_z}}\nabla^2\psi + \frac{k_z}{n_0}\Delta n(r,z)\psi$$

For a rotating astigmatic quadratic duct:

$$\Delta n(r,z) = \alpha(x^2+y^2) + \epsilon[(x\cdot\cos\beta z - y\cdot\sin\beta z)^2 - (x\cdot\sin\beta z + y\cdot\cos\beta z)^2]$$

with the identification $z \to \frac{t}{\hbar k_z n_0}$, $\alpha \to \frac{1}{2}m\omega^2$, $\frac{k_z}{n_0}\epsilon \to \frac{1}{2}m\omega^2\epsilon$, and $m = (\hbar k_z n_0)^2$, $\Omega = \frac{\beta}{\hbar k_z n_0}$, we arrive at a Schrodinger equation:

$$i\partial_t\psi = H\psi = \frac{\hbar^2}{2m}\nabla^2\psi + \frac{1}{2}m\omega^2[(x^2+y^2) + \epsilon\{(x\cdot\cos\Omega t - y\cdot\sin\Omega t)^2 - (x\cdot\sin\Omega t + y\cdot\cos\Omega t)^2\}]$$

To remove the time-dependence from the Hamiltonian $H$, we apply a time-dependent unitary transformation to move to a frame that rotates with the duct: $U(t) = \exp\left(i\frac{\Omega\, L_z t}{\hbar}\right)$.

The Hamiltonian then reads:

$$H_{rot} = \frac{\hbar^2}{2m}\nabla^2 + \frac{1}{2}m[(\omega^2-\Omega^2)r^2 + \epsilon\,\omega^2\,(x^2-y^2)] + \Omega L_z$$

One might conclude from the form of the Hamiltonian that the $L_z$ term immediately breaks time reversal symmetry even without any trap astigmatism ($\epsilon = 0$). This clearly cannot be the case, as for an astigmatism-free trap, the Hamiltonian actually has no time-dependence. It may be understood mathematically by considering the first two excited trap-states $\psi_{10} = \mathrm{LG}_{10} \equiv \mathrm{HG}_{10} + i\mathrm{HG}_{01}$ and $\psi_{01} = \mathrm{LG}_{01} \equiv \mathrm{HG}_{10} - i\mathrm{HG}_{01}$, which are Laguerre-Gauss (LG) modes with orbital angular momenta of $+\hbar$ and $-\hbar$ about the origin (respectively), and no radial nodes, written in terms of the Hermite-Gauss (HG) modes. In the rotating frame, the energy splitting between these two states is evidently $2\hbar\Omega$. It is important to remember that the original Hamiltonian is a *Floquet* Hamiltonian, which periodically drives the system with a frequency of $\Omega$; consequently, the resulting quasi-energy spectrum of the system repeats every $\hbar\Omega$ in energy (or more precisely is only defined modulo $\hbar\Omega$ in energy), much as the dispersion of a spatially-periodic lattice system repeats every $\hbar/a$ in momentum, where $a$ is the lattice spacing. This means that our splitting of $2\hbar\Omega$ is equivalent to *no splitting at all.*

To induce a splitting between $\psi_{10}$ and $\psi_{01}$, it is *essential* that the trap be astigmatic, so that its rotation can inject angular momentum and thus break time-reversal symmetry. If the astigmatism is large compared to the rotation rate ($\omega\left[\sqrt{1+\epsilon} - \sqrt{1-\epsilon}\right] \approx \omega\,\epsilon \gg \Omega$), then the modes are mostly **x**- and **y**- HG-like, rather than the desired LG modes. The desirable limit is $\Omega \gg \omega\,\epsilon$, corresponding to rotation fast compared to astigmatism (though *not* large compared to the

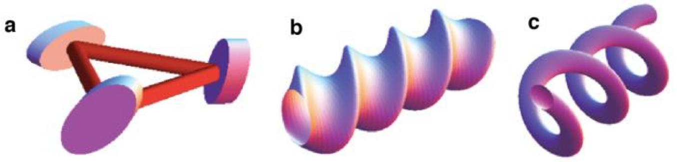


**Figure S6. a,** An astigmatic three mirror resonator may produce an effective magnetic field for light. **b,** A twisting waveguide, which is similar to the three mirror astigmatic resonator, may also produce an effective magnetic field. Because it uses astigmatism to stir the light, the mechanism for destroying the Landau level comes in at the same order as the mechanism that creates it. **c,** A writhing waveguide, which is more similar to a four mirror non-planar resonator, also may create a synthetic magnetic field, but it also fails to produce a stable Landau level. Both the twisting and the writhing waveguides are promising routes for producing a synthetic field as long as the Landau level regime is not desired.

*average* trapping frequency $\omega$). In this limit the astigmatism induces a small additional splitting $\frac{\epsilon^2\omega^2}{4\Omega}$ which persists even once we transform back to the lab frame.

As the rotation frequency $\Omega$ approaches harmonic trapping frequency $\omega$, the lowest Landau level begins to form, in the sense that all states $\psi_{l0}$, for $l \geq 0$, approach degeneracy. At this point the astigmatism which was employed to break the degeneracy between $\psi_{l0}$ and $\psi_{0l}$ (among other states) becomes problematic, in that it begins to couple states with $\Delta l = 2$, within the lowest Landau level; this corresponds to a saddle trap and the deconfinement of all eigenstates.

There is thus an optimal amount of astigmatism; too little and time reversal symmetry will not be broken, but as the rotation frequency approaches the centrifugal limit, excessive astigmatism results in eigenstate deconfinement.

To see these relations more formally, we rewrite the Hamiltonian in terms of raising operators for quantized trap excitations along x and y (in the limit of small $\epsilon$):

$$\frac{H}{\hbar} = \omega\left(a_x^\dagger a_x + a_y^\dagger a_y\right) + i\,\Omega\left(a_x^\dagger a_y - a_y^\dagger a_x\right) + \omega\epsilon\left(a_x^\dagger a_x - a_y^\dagger a_y\right) + \omega\frac{\epsilon}{2}\left(a_x^2 + a_x^{\dagger^2} - a_y^2 - a_y^{\dagger^2}\right)$$

Switching to the basis of quantized excitations with well-defined angular momentum ($a_{\{l,r\}}^\dagger = \frac{a_x^\dagger \pm i\, a_y^\dagger}{\sqrt{2}}$), we arrive at:

$$\frac{H}{\hbar} = (\omega + \Omega)a_r^\dagger a_r + (\omega - \Omega)a_l^\dagger a_l + 2\omega\epsilon\left(a_l^\dagger a_r + a_r^\dagger a_l\right) + \omega\epsilon\left(a_l^{\dagger^2} + a_l^2 + a_r^{\dagger^2} + a_r^2\right)$$

As $\Omega$ approaches $\omega$, the energy cost of adding an $l$ excitation goes to zero, corresponding to the creation of Landau levels, where $a_l^\dagger a_l$ is the angular momentum about the center, and $a_r^\dagger a_r$ is the index of the Landau level. The term $\omega\epsilon\left(a_l^\dagger a_r + a_r^\dagger a_l\right)$ breaks time reversal symmetry by mixing the Landau levels weakly, as above (shifting the trapping frequency by $\frac{\epsilon^2\omega^2}{\Omega}$; this can be compensated by a slight change in $\omega$ or $\Omega$). As $\Omega$ approaches $\omega$, the cost to add or remove two $l$ excitations goes to zero, allowing the final term $\omega\epsilon\left(a_l^{\dagger^2} + a_l^2 + a_r^{\dagger^2} + a_r^2\right)$ to mix all of the states within each Landau level at no energy cost, thus destroying the flatness of the Landau levels.

In essence, the lowest Landau level lives on a saddle potential induced by the astigmatism that was necessary to break time-reversal, and all states in the lowest Landau level become unconfined edge states of the saddle. This is the origin of the centrifugal limit in astigmatic traps.

*Writhing Waveguide:*

In the case of a *circular* quadratic duct whose center is translating in space, we have a similar Hamiltonian to that of twist, except that the index of refraction may be written as: $\Delta n(r,z) = \alpha[(x - r_0 \cdot \cos\beta z)^2 + (y - r_0 \cdot \sin\beta z)^2]$, where $r_0$ is the radius of the orbit of the duct. Again moving to the frame of the instantaneous eigenstates, we employ the same unitary operator $U_{rot} = e^{i\Omega L_z t/\hbar}$, which now provides an effective Hamiltonian (with $\beta z \rightarrow \Omega t$):

$$H_{rot} = \frac{\hbar^2}{2m}\nabla^2 + \frac{1}{2}m[\omega^2(x - r_0)^2 + \omega^2 y^2 - \Omega^2 r^2] + \Omega L_z$$

At first glance, this Hamiltonian seems to be astigmatism free; the only issue is that the harmonic trap is not centered on the same location as the origin of $L_z$. To move the trap to the origin we now apply the unitary translation operator $U_{trans} = e^{i\, p_x r_0}$, which, it should be noted, does not commute with $L_z$. The resulting Hamiltonian is:

$$H_{rot} = \frac{\hbar^2}{2m}\nabla^2 + \frac{1}{2}m(\omega^2 - \Omega^2)r^2 + \hbar\Omega L_z + \Omega\, r_0 p_y$$

$$= \frac{p^2}{2m} + \frac{1}{2}m(\omega^2 - \Omega^2)r^2 + \hbar\Omega L_z + \Omega\, r_0 p_y$$

We now switch to the basis of quantized angular excitations, in which the Hamiltonian reads:

$$H_{rot}/\hbar = (\omega + \Omega)a_r^\dagger a_r + (\omega - \Omega)a_l^\dagger a_l + \Omega r_0\sqrt{\hbar m\omega}(a_l^\dagger + a_l - a_r^\dagger - a_r)$$

It is apparent that the term $(a_r^\dagger + a_r)$ breaks time reversal, as in the twisted waveguide, by mixing the Landau levels. The term $(a_l^\dagger + a_l)$ mixes the states within the lowest Landau level, breaking its flatness. The state mixing does not arise from a saddle potential, but nonetheless inextricably ties time-reversal symmetry breaking to destruction of the lowest Landau level.

In the twisting and writhing waveguides (as in rotating BECs, etc…) the breaking of time-reversal symmetry is inextricably tied to destruction of the lowest Landau level: you cannot have one without the other, as the perturbation which induces the stirring (that breaks time-reversal) must break rotational symmetry. This should be compared to the non-planar resonator, where geometric rotations on each round-trip provide the necessary chirality, without needing to break rotational invariance.

**14. A note on time reversal symmetry in our system** Our system does not break time reversal symmetry—the resonator photons are analogous to electrons in a spin-hall system where the up/down spin degree of freedom is direction of propagation through the resonator. Modes travelling in opposite directions experience opposite round trip rotations and therefore opposite effective magnetic fields. So, any desired mode has a corresponding degenerate back-reflected mode. However, the polarization of the light is rotated along with the image, so the back-reflected mode has the opposite circular polarization. Therefore, future experiments may exploit the atomic Faraday effect by placing a cloud of optically pumped Rubidium atoms in the resonator waist in order to split the polarization modes and the break time reversal symmetry of our system.


31 Zupancic, P. P. J. *Dynamic Holography and Beamshaping using Digital Micromirror Devices* Masters thesis, Ludwig-Maximilians-Universitat Muchen, (2013).

32 Girvin, S. M. The Quantum Hall Effect: Novel Excitations and Broken Symmetries. *arXiv:cond-mat/9907002* (1999).

33 Dean, C. R. *et al.* Hofstadter/'s butterfly and the fractal quantum Hall effect in moire superlattices. *Nature* **497**, 598-602, doi:10.1038/nature12186 (2013).

34 Hofstadter, D. R. Energy levels and wave functions of Bloch electrons in rational and irrational magnetic fields. *Phys. Rev. B* **14**, 2239-2249, doi:10.1103/PhysRevB.14.2239 (1976).

35 Hasan, M. Z. & Kane, C. L. Colloquium: Topological insulators. *Rev. Mod. Phys.* **82**, 3045-3067, doi:10.1103/RevModPhys.82.3045 (2010).

36 Lin, Y. J., Compton, R. L., Jiménez-García, K., Porto, J. V. & Spielman, I. B. Synthetic magnetic fields for ultracold neutral atoms. *Nature* **462**, 628-632, doi:10.1038/nature08609 (2009).
37 Abo-Shaeer, J. R., Raman, C., Vogels, J. M. & Ketterle, W. Observation of Vortex Lattices in Bose-Einstein Condensates. *Science* **292**, 476-479, doi:10.1126/science.1060182 (2001).
38 Yarmchuk, E. J., Gordon, M. J. V. & Packard, R. E. Observation of Stationary Vortex Arrays in Rotating Superfluid Helium. *Phys. Rev. Lett.* **43**, 214-217, doi:10.1103/PhysRevLett.43.214 (1979).
39 Goldstein, H., Jr, C. P. P. & Safko, J. L. *Classical Mechanics*. 3 edition edn, (Addison-Wesley, 2001).
40 Ho, T.-L. Bose-Einstein Condensates with Large Number of Vortices. *Phys. Rev. Lett.* **87**, 060403 (2001).
41 Siegman, A. E. *Lasers*. (University Science Books, 1986).
42 Aidelsburger, M. *et al.* Realization of the Hofstadter Hamiltonian with Ultracold Atoms in Optical Lattices. *Phys. Rev. Lett.* **111**, doi:10.1103/PhysRevLett.111.185301 (2013).
43 Miyake, H., Siviloglou, G. A., Kennedy, C. J., Burton, W. C. & Ketterle, W. Realizing the Harper Hamiltonian with Laser-Assisted Tunneling in Optical Lattices. *Phys. Rev. Lett.* **111**, doi:10.1103/PhysRevLett.111.185302 (2013).
44 Habraken, S. J. M. & Nienhuis, G. Modes of a twisted optical cavity. *Phys. Rev. A* **75**, doi:10.1103/PhysRevA.75.033819 (2007).
45 Laughlin, R. B. Anomalous Quantum Hall Effect: An Incompressible Quantum Fluid with Fractionally Charged Excitations. *Phys. Rev. Lett.* **50**, 1395-1398, doi:10.1103/PhysRevLett.50.1395 (1983).
46 Bernevig, B. A. & Haldane, F. D. M. Model Fractional Quantum Hall States and Jack Polynomials. *Phys. Rev. Lett.* **100**, 246802 (2008).
47 Jia, N. *et al.* Observation of Cavity Rydberg Polaritons. *arXiv: 1511.01872* (2015).
48 Beterov, I. I., Ryabtsev, I. I., Tretyakov, D. B. & Entin, V. M. Quasiclassical calculations of blackbody-radiation-induced depopulation rates and effective lifetimes of Rydberg $nS$, $nP$, and $nD$ alkali-metal atoms with $n\ensuremath{\le}80$. *Phys. Rev. A* **79**, 052504 (2009).
49 Douglas, M. & Klevtsov, S. Bergman Kernel from Path Integral. *Commun. Math. Phys.* **293**, 205-230, doi:10.1007/s00220-009-0915-0 (2010).
50 Habraken, S. J. M. & Nienhuis, G. Stability properties of a rotating astigmatic optical cavity. *Proc. SPIE 7227, Complex Light and Optical Forces III*, 72270H (2009).
51 Mamaev, A. V. & Saffman, M. Optical Vortex Patterns in a Unidirectional ring Oscillator. *Physica Scripta.* **1996**, 21 (1996).
52 Chiao, R. Y. *et al.* Observation of a topological phase by means of a nonplanar Mach-Zehnder interferometer. *Phys. Rev. Lett.* **60**, 1214-1217, doi:10.1103/PhysRevLett.60.1214 (1988).
53 Nilsson, A. C., Gustafson, E. K. & Byer, R. L. Eigenpolarization theory of monolithic nonplanar ring oscillators. *IEEE Journal of Quantum Electronics* **25**, 767-790, doi:10.1109/3.17343 (1989).
54 Scheeler, M. W., Kleckner, D., Proment, D., Kindlmann, G. L. & Irvine, W. T. M. Helicity conservation by flow across scales in reconnecting vortex links and knots. *PNAS* **111**, 15350-15355, doi:10.1073/pnas.1407232111 (2014).

55 Firstenberg, O. *et al.* Attractive photons in a quantum nonlinear medium. *Nature* **502**, 71-75, doi:10.1038/nature12512 (2013).
56 Bajcsy, M. *et al.* Efficient All-Optical Switching Using Slow Light within a Hollow Fiber. *Phys. Rev. Lett.* **102**, doi:10.1103/PhysRevLett.102.203902 (2009).
